# Supplementary material for: Dynamic Approaches to In-Network Aggregation
Source: arXiv:0810.3227 source file (2008-10-17)
Supplement: Supplementary file 1 [file sec_appendix.tex]

We now analyze the behavior of push-sum given these changes.  As in the analysis of push-sum, we begin by analyzing the behavior of the potential function $\Phi_t$.  Given host $j$'s value contribution to host $i$'s value $v_{i,j} \in [0,1]$ and host $i$'s weight $w_{i} \in (0,n]$, the systemwide potential is 
$$\Phi_t = \sum_{i,j}(v_{i,j} - \frac{w_{i}}{n}) = \sum_{i,j}\rho_{i,j}^2$$

The communication assignment function $f$ is defined such that at time $t$ host $k$ randomly selects host $f(k)$ to send mass to.  We also define the test and indegree functions ($u_i$ and $g$ respectively).
$$u_i(j) = \left\{\begin{array}{cc}j = i & 1 \\j \neq i & 0\end{array}\right.$$
$$g(i) = |\{k|f(k) = i\}|+1$$

Given the unmodified potential function $\Phi$ as described by Kempe, the modified potential $\Phi^*$ at $t+1$ is
$$\Phi_{t+1}^* = \sum_{i,j} \left[((1-\lambda) v_{i,j} - \frac{(1-\lambda)w_i+\lambda}{n}) + \lambda \right.$$
$$\left.+\sum_{k:f(k) = i} ((1-\lambda) v_{k,j} - \frac{(1-\lambda)w_k+\lambda}{n})\right]$$
$$=\sum_{i,j}\left(\frac{1-\lambda}{2}\rho_{i,j} + \lambda u_i(j) -\frac{g(i)\lambda}{2n}+ \sum_{k:f(k) = i}\frac{1-\lambda}{2}\rho_{k,j} \right)^2$$

$$= \sum_{i,j}\frac{(1-\lambda)^2}{4}\rho_{i,j}^2 + \sum_{i,j,k:f(k)=i}\frac{(1-\lambda)^2}{4}\rho_{k,j}^2$$
$$+\frac{(1-\lambda)^2}{2}\sum_{i,j,k:f(k)=i}\rho_{i,j}\rho_{k,j}$$
$$+\frac{(1-\lambda)^2}{2}\sum_{i,j,k\neq k':f(k')=f(k)=i}\rho_{k',j}\rho_{k',j}$$
$$+\sum_{i}\lambda^2-\frac{\lambda^2}{4n^2}\sum_{i,j} g^2(i)$$
$$+(\lambda-\lambda^2)\sum_i\rho_{i,i} - \frac{\lambda-\lambda^2}{2n}\sum_{i,j}\rho_{i,j}g(i) $$
$$+(\lambda-\lambda^2)\sum_i\sum_{k:f(k)=i}\rho_{k,i} - \frac{\lambda-\lambda^2}{2n}\sum_{i,j}\sum_{k:f(k)=i}\rho_{k,j}g(i)$$

%$$= \Phi_{t+1} +\lambda^2\sum_{i}(1-\frac{g^2(i)}{4n})$$
%$$+(\lambda-\lambda^2)\sum_i(\rho_{i,i} + \sum_{k:f(k)=i}\rho_{k,i})$$
%$$- \frac{\lambda-\lambda^2}{2n}\sum_{j}\left[(\sum_{i}g(i)\rho_{i,j}) + (\sum_{k}g(k)\rho_{k,j})\right]$$

$$= (1-\lambda)^2\Phi_{t+1} +\lambda^2\sum_{i}(1-\frac{g^2(i)}{4n})$$
$$+(\lambda-\lambda^2)\sum_i\left[(v_{i,i} - \frac{w_i}{n}) + \sum_{k:f(k)=i} (v_{k,i} - \frac{w_k}{n})\right]$$
$$- \frac{\lambda-\lambda^2}{2n}\sum_{j,i}g(i) \left[(v_{i,j} - \frac{w_i}{n}) + \sum_{k:f(k)=i} (v_{k,j} - \frac{w_k}{n})\right]$$

%XXX get some proof!  These exepectations converge here... but what's the deal with g^2
The indegree function $g(i)$ is the number of hosts that send mass to host $i$ (note that all hosts have a loopback edge).  Since each is selected independently, by the continual limit theorem this is a normal distribution for high $n$, and $E[g(i)] =2$ and $E[g^2(i)] = 5$.
$$E[\Phi_{t+1}^*|\Phi_t^* = \phi]$$

$$= (1-\lambda)^2(\frac{1}{2} - \frac{1}{2n})\phi +\lambda^2\sum_{i}(1-\frac{E[g^2(i)]}{4n})$$
$$+(\lambda-\lambda^2)\sum_i\left[(v_{i,i} - \frac{w_i}{n}) + \sum_{k} (v_{k,i} - \frac{w_k}{n})P[f(k)=i]\right]$$
$$- \frac{\lambda-\lambda^2}{2n}\sum_{j,i} \left[(v_{i,j} - \frac{w_i}{n}) + \sum_{k:f(k)=i} (v_{k,j} - \frac{w_k}{n})\right]E[g(i)]$$
